# Supplementary material for: Flatness and Complexity of Immediate Observation Petri Nets
Source: arXiv:2001.09966 source file (2020-07-21)
Supplement: Supplementary file 2 [file appendix-complexity.tex]

%!TEX root = main.tex
We recall Proposition 5 of a previous paper~\cite{conf/concur/EsparzaGMW18}.
It shows that a boolean combination of counting sets is still a counting set and gives bound on the norms of counting constraints representing these combinations.

\begin{proposition}[Proposition 5 of~\cite{conf/concur/EsparzaGMW18}]
\label{prop:oponconf}
Let $\cC_1, \cC_2$ be counting constraints.
\begin{itemize}
\item There exists a counting constraint $\cC$ with $\sem{\cC} = \sem{\cC_1} \cup \sem{\cC_2}$ such that
$\unorm{\cC} \leq \max \{\unorm{\cC_1}, \unorm{\cC_2} \}$ and $\lnorm{\cC} \leq \max \{\lnorm{\cC_1}, \lnorm{\cC_2} \}$.
\item  There exists a counting constraint $\cC$ with $\sem{\cC} = \sem{\cC_1} \cap \sem{\cC_2}$ such that
$\unorm{\cC} \leq \unorm{\cC_1} + \unorm{\cC_2}$ and $\lnorm{\cC} \leq \lnorm{\cC_1} + \lnorm{\cC_2}$.
\item There exists a counting constraint $\cC$ with $\sem{\cC} = \N^n \setminus \sem{\cC_1}$ such that
$\unorm{\cC} \leq n\lnorm{\cC_1}$ and $\lnorm{\cC} \leq n\unorm{\cC_1} + n$.
\end{itemize}
 \end{proposition}

To prove Lemma \ref{lemma:bio-cube-preimage} that bounds the pre-image of a counting set, 
we first prove a result bounding the pre-image of a single marking of a \bio{} net.

\begin{lemma}
\label{lemma:bio-point-preimage}
Let $\targetMarking$ be a marking of size $\targetSize$.
The pre-image $\prestar(\targetMarking)$ is a counting set and its norm is bound by 
 \begin{align*}
\unorm{\pre^*(\targetMarking)} \leq \placeCount (\targetSize + \placeCount)
 \text{ and }
\lnorm{\pre^*(\targetMarking)} \leq  \placeCount (\targetSize + \placeCount).
 \end{align*}
\end{lemma}
\begin{proof}
We show that the token counts above 
$\targetSize + \placeCount$
are not distinguishable from the point of view of reachability
of $\targetMarking$.

Let $\dec{H}$ be a realizable decorated history such that $\sourceMarking \trans{\dec{H}} \targetMarking$.
Recall that this decorated history always exists, by definition of realizability and the fact that the decoration with zero smoke nodes always exists.
By the repeated application of the Replacement Lemma, we can assume that $\dec{H}$ is  fuel-efficient.

By Lemma \ref{lm:blue-irrelevance}, 
there exists a realizable decorated history $\dec{H}'$ from a marking $M''$ to $\targetMarking$ 
for any marking $M''$ such that
$\sourceMarking$ in $\dec{H}$ and $M''$ in $\dec{H}'$ have the same multisets of places labelling their cargo and fuel nodes, 
and the support of the labels of $M''$'s smoke nodes is included in the support of the labels of $\sourceMarking$'s smoke nodes.
Therefore, any such $M''$ belongs to $\prestar(\targetMarking)$.

Thus
\cwk{is this thus clear enough?}
 $\prestar(\targetMarking)$ is a counting set as a union of cubes 
with bounds on places $p$ of the form 
$a \leq p \leq a$ for $a \in \set{0,\ldots,\targetSize + \placeCount}$ and
$1 \leq p \leq \infty$, 
of which there are a finite number.
\end{proof}

Now we can prove Lemma \ref{lemma:bio-cube-preimage} by reducing the problem to an application of Lemma \ref{lemma:bio-point-preimage}.

\BIOCubePreimage*
\begin{proof}
Every cube $\cube$ can be decomposed into a finite union of
what we call in this proof
\emph{simple cubes}: cubes
with bounds on each place $p$ of the form 
$a_p \leq p \leq a_p$ and
$b_p \leq p \leq \infty$ 
for some $a_p,b_p \in \N$.
The lower bounds $L$ of these simple cubes are bound by the addition of all the highest bounds used to define $\cube$, \ie $|L| \leq \unorm{\cube}+\lnorm{\cube}$.

Let $\cube$ be a cube.
%Without loss of generality, we can 
Assume that $\cube$ is a simple cube as described above.
For each place $p$ with upper bound $\infty$, we add a transition $t$
with preset $\preset{t}=\set{p}$ and postset $\postset{t}=\emptyset$.
It is easy to see that for every marking $\sourceMarking$,
the modified net $\net'$ has a firing sequence
from $\sourceMarking$ to the lower bound $L$ of $\cube$ 
iff
the original net $\net$ has a firing sequence from $\sourceMarking$ to some marking in
$\cube$.
It then remains to apply Lemma~\ref{lemma:bio-point-preimage} to $L$ and $\net'$, which has the same place count
%, maximal observation degree and maximal output degree 
as $\net$.
If $\cube$ is actually a union of simple cubes, then the bounds still apply as the norm of a union is the maximum of the norms.
\end{proof}

Lemma \ref{lemma:bio-cube-preimage} allows us to prove the following strong result.
It is similar to a result for IO nets
from the proof of Theorem 4.50 of \cite{journals/corr/abs-1912-06578}.
%The proof is almost identical to the original proof,
%and is supplied in the appendix.
%for the sake of completeness.

\begin{theorem}
\label{thm:pspace-lemma}
Let $\mathcal{S}_1$ and $\mathcal{S}_2$ be two functions 
that take as arguments a \bio{} net $\net$ and a finite list of counting constraints $X$,
and return counting sets $\mathcal{S}_1(\net,X)$ and $\mathcal{S}_2(\net,X)$ respectively.

Assume that $\mathcal{S}_1(\net,X)$  and $\mathcal{S}_2(\net,X)$ 
have
norms at most exponential in the size of $(\net,X)$,
as well as
\PSPACE{}-decidable membership
(given input $(\targetMarking,\net,X)$,
decide whether $\targetMarking\in \mathcal{S}_i(\net,X)$).

Then the same is true about the counting sets
$\mathcal{S}_1(\net,X)\cap\mathcal{S}_2(\net,X)$,
$\mathcal{S}_1(\net,X)\cup\mathcal{S}_2(\net,X)$,
$\compl{\mathcal{S}_1(\net,X)}$,
$\prestar(\mathcal{S}_1(\net,X))$.
Furthermore the emptiness of the aforementioned sets is decidable in \PSPACE{}, given input $(\net,X)$.
\end{theorem}
\begin{proof}
The exponential bounds for the norms follow immediately from 
the norms of set-theoretical combinations of counting constraints in Proposition \ref{prop:oponconf},
and Lemma~\ref{lemma:bio-cube-preimage}.
The membership complexity for union, intersection and
complement is easy to see.
It remains to demonstrate that the complexity of membership in
$\prestar(\mathcal{S}_1(\net,X))$
can be decided in \PSPACE.

By Savitch's Theorem, \NPSPACE=\PSPACE, so it is sufficient to provide a nondeterministic algorithm.
Given $(\sourceMarking,\net,X)$,
we want to decide whether $\sourceMarking\in\prestar(\mathcal{S}_1(\net,X))$.
%By Lemma~\ref{lemma:bimo-cube-preimage}, we know that minimal markings of $\prestar(\mathcal{S}_1(\net,X))$ have at most 
%$K\defeq \placeCount(\unorm{\mathcal{S}_1(\net,X)}+ \lnorm{\mathcal{S}_1(\net,X)} +\maxObservation)(\placeCount+2)^\placeCount)$ tokens.
As in the proof of Lemma~\ref{lemma:bio-cube-preimage}, it is enough to check that $\sourceMarking$ can reach a marking of size $\unorm{\mathcal{S}_1(\net,X)}+ \lnorm{\mathcal{S}_1(\net,X)}$ in $\mathcal{S}_1(\net,X)$ in a modified net with a few extra (destroying) transitions.
%The algorithm 
%constructs $M''$ such that $M''(p)=\min(\sourceMarking(p),K$ for all places $p$.
%reduces the token counts in $\sourceMarking$
%to at most
%$(\unorm{\mathcal{S}_1(\net,X)}+ \lnorm{\mathcal{S}_1(\net,X)} +\maxObservation)(\placeCount+2)^\placeCount$
%tokens for each place.
The algorithm 
%then
guesses a firing sequence 
in this modified net
starting at $\sourceMarking$, step by step,
guessing each time a marking of size bound 
%by Lemma \ref{lemma:bimo-intermediate-values}
by the Shortening Theorem
 with $\sourceSize \defeq |\sourceMarking|$ and $\targetSize \defeq \unorm{\mathcal{S}_1(\net,X)}+ \lnorm{\mathcal{S}_1(\net,X)}$,
%while keeping track of places having enough tokens to become \red,
%ignoring the exact token counts in the \red{} places,
and
checking after each step if the reached configuration
is in $\mathcal{S}_1(\net,X)$.

At every moment we store descriptions of two configurations,
the current one and the next one, which can be done in polynomial space
%for the same reasons as in Theorem~\ref{thm:bimo-reachability}.
as they are 
of size exponential in the size of the input $(\sourceMarking,\mathcal{S}_1(\net,X),\net)$, 
where $\mathcal{S}_1(\net,X)$ also has size exponential in the input.
%of size polynomial in $\sourceSize, \unorm{\mathcal{S}_1(\net,X)}, \lnorm{\mathcal{S}_1(\net,X)}, \maxObservation, \outputDegree$ and exponential in $\placeCount$, and $\mathcal{S}_1(\net,X)$ has norms exponential in $(\net,X)$. 

If a counting set is of exponential norm, then it contains \PSPACE{} describable markings and thus checking emptiness is done by simply guessing such a marking and checking whether it is in the set. 
\end{proof}

Theorem \ref{thm:pspace-lemma} allows us to verify a wide range of properties for \bio{} nets in \PSPACE.
For example, the results for cubes that could be solved in IO are still solvable for \bio. 

\TheoremBioCube*

\begin{proof}
These problems are \PSPACE-hard because they are \PSPACE-hard for IO nets, which are a subclass of \bio{} nets.

For the following problems, let $\net$ be a \bio{} net, and $\cube', \cube$ two cubes.
%Recall that by Savitch's Theorem, \NPSPACE=\PSPACE, so it is sufficient to provide a nondeterministic algorithm.

\textbf{Reachability.}
Cube $\cube'$ can reach $\cube$ if and only if $\cube' \cap \prestar(\cube)$ is non empty.
By Theorem~\ref{thm:pspace-lemma},
this is solvable in \PSPACE{} in the size of $\net$ and $X \defeq \cube',\cube$.
%By Lemma~\ref{lemma:bimo-cube-preimage}, we know that two markings 
%differing only in places with more than 
%$K\defeq \placeCount\times max(\unorm{\cube}+ \lnorm{\cube},\maxObservation)\placeCount^\placeCount)$ 
%tokens are indistinguishable from the  point of view of reachability  to  cube $\cube$.
%By Savitch's Theorem, \NPSPACE=\PSPACE, so it is sufficient to provide a nondeterministic algorithm.
%We nondeterministically guess a marking $\sourceMarking$ in $\cube'$ with  at most $K$ tokens in each place,
%and which is therefore describable in \PSPACE.
%We simply check  its membership in $\prestar(\cube)$, which is \PSPACE-decidable by Theorem~\ref{thm:pspace-lemma}. 

\textbf{Coverability.} 
Cube $\cube'$ covers cube $\cube$ if and only if the upward closure of $\cube$ is reachable from $\cube'$. 
The upward closure of $\cube$ is still a counting set (we just replace all upper bounds by $\infty$) of norms at most the norms of $\cube$.
By the above paragraph on reachability, this problem is solvable \PSPACE.

\textbf{Liveness.} 
Let $t$ be a transition of $\net$.
The set $En(t)$ of markings that enable $t$ contains the markings that put at least one token in the source place (if there is one) and at least the multiset of necessary tokens in the observed places. Clearly, $En(t)$ is a cube.
Then $\overline{\pre^*(En(t))}$ is the set of markings $M$ from which one cannot execute 
transition $t$ anymore by any firing sequence starting in $M$. So the set $\mathcal{L}$ of live markings of $\net$ is given by
$$
\mathcal{L} = \overline{ \pre^*\left( \bigcup_{t \in T} \overline{\pre^*(En(t))} \right) }
$$
Deciding whether $\cube \subseteq \mathcal{L}$ is equivalent to deciding whether  $\cube \cap \overline{\mathcal{L}} = \emptyset$ holds.
By Theorem \ref{thm:pspace-lemma} 
%we are dealing with counting sets of exponential norm, with \PSPACE-decidable membership.
%If a counting set is of exponential norm, then it contains \PSPACE{} describable markings and thus checking emptiness is done by simply guessing such a marking and checking whether it is in the set.
%Thus the cube-liveness problem 
this
can be solved in \PSPACE \ in the size of the input, i.e. net $\net$ and cube $\cube$.
\end{proof}
